# Supplementary material for: Efficient and High-quality Prehensile Rearrangement in Cluttered and Confined Spaces
Source: arXiv:2110.02814 source file (2022-03-18)
Supplement: Supplementary file 1 [file 07_appendix.tex]

\section{Appendix}
\label{sec:appendix}
